# Supplementary material for: A Passivity-based Approach for Variable Stiffness Control with Dynamical Systems
Source: arXiv:2307.09571 source file (2023-07-18)
Supplement: Supplementary file 1 [file Appendix.tex]

\appendix[Solution of the optimization problem~\eqref{eq:LS_inversion_solution}] 
By setting $h=1$ and omitting for simplicity the indexes $t$ and $d$, the optimization problem~\eqref{eq:LS_inversion_solution} can be written as
\begin{equation}
    \begin{split}
        &\min_{\hat{\bfu}} \frac{1}{2}\Vert \bfv_{c} + \hat{\bfL}^{+}\lambda \bfe - \hat{\bfL}^{+} \hat{\bfu} \Vert^2 = \\
        &\min_{\hat{\bfu}} \frac{1}{2}\Vert \bfy - \hat{\bfL}^{+} \hat{\bfu} \Vert^2 ,
    \end{split}
    \label{eq:LS_inversion_rewrite}
\end{equation}
where we set $\bfy = \bfv_{c} + \hat{\bfL}^{+}\lambda \bfe$. The problem~\eqref{eq:LS_inversion_rewrite} is now in the typical least-square form and the solution can be computed my means of the pseudo-inverse of $\hat{\bfL}^{+}$ as~\cite{bishop2006pattern}
\begin{equation}
    \hat{\bfu} = \left(\hat{\bfL}^{+}\right)^{+}\bfy = \hat{\bfL} \left(\bfv_{c} + \lambda \hat{\bfL}^{+} \bfe\right),
\end{equation}
where we used the property $\left(\hat{\bfL}^{+}\right)^{+} = \hat{\bfL}$.
